# Supplementary material for: Hydrodynamics of quartz crystal microbalance experiments with liposome-DNA complexes
Source: arXiv:2002.12141 source file (2020-02-21)
Supplement: Supplementary file 1 [file SI5.pdf]

# Supplementary information: Hydrodynamics of quartz crystal microbalance experiments with liposome-DNA complexes

Adolfo Vazquez-Quesada,[1] Marc Melendez Schofield,[1] Achilleas Tsortos,[2] Pablo Mateos-Gil,[2] Electra Gizeli,[2,3] and Rafael Delgado Buscalioni[1,*]

[1]*Departmento de Fisica de la Materia Condensada, Universidad Autonoma de Madrid, and Institute for Condensed Matter Physics, IFIMAC. Campus de Cantoblanco, Madrid 28049, Spain*

[2]*Institute of Molecular Biology and Biotechnology, Foundation for Research and Technology-Hellas, Heraklion, Crete, 70013, Greece*

[3]*Department of Biology, University of Crete, Heraklion 71110, Greece*

PACS numbers:

## EXPERIMENTS

Experiments with liposome-DNA (LDNA) complexes were performed using a QCM-D setup (Q-Sense E4, Sweden) capable of measuring changes in resonance frequency $\Delta f$) and energy dissipation ($\Delta D$). Measurements reported here were performed at operating frequency of 35 MHz (i.e. 7th harmonic), with continuous flow rate of 60 l/min and fixed temperature of 25$^o$C. A more detailed description of acoustic measurements is reported elsewhere [1]. Figure 1 (A) shows a typical sensogram depicting the formation of LDNA complex in real time. The figure illustrates the changes in $\Delta f$ (black) and $\Delta D$ (green) signals recorded upon sequential injections of (i) neutravidin (NAv), (ii) DNA, and (iii) POPC liposomes. Plateau values corresponding to frequency and dissipation changes registered after addition of liposomes were used to calculate the acoustic ratio of the LDNA complex as $\Delta D_{\rm LDNA}/\Delta f_{\rm LDNA}$. In addition, dissipation capacity (DC) of LDNA complexes, i.e. lim $(\Delta D/\Delta f)_{\rm LDNA}$ when $\Delta f_{\rm LDNA} \to 0$, were derived using real time graphs. Figure 1(B) plots the calculated $(\Delta D/\Delta f)_{\rm LDNA}$ against the corresponding amount of liposomes on the surface, i.e. $\Delta f_{\rm LDNA}$, for the all the points of the sensogram since the onset of regime (iii) in panel A (from minute 32 to minute 38 in panel A). The red line indicates the method used to obtain the DC of LDNA complexes, which is taken as the intercept $\Delta f_{\rm LDNA} \to 0$ (marked with an asterisk). All reported measurements of $\Delta f$ are used as raw data, i.e., without dividing them by the number of the harmonic

## NUMERICAL MODEL

### Fluid solver

Our numerical model is based on a fluctuating hydrodynamic solver for compressible flow equipped with an immersed boundary method to couple the fluid and structure dynamics. A detailed explanantion of the method can be found in Refs. [2–4]. The code is called `FLUAM` is written in CUDA and runs on GPU architectures, it is available at a github repository [5]. The integration scheme is second-order accurate in space and time and the spatial discretization is based on a staggered grid [6] of size $h$. Boundary conditions for the top and bottom walls are imposed using a ghost cell [4]. This enables us to easily impose a tangential flow velocity at the bottom wall. The tangential velocity gradient at the wall cells $(\partial v_x/\partial y)_{y=0}$ is calculated using second order interpolation from the values of the fluid cell velocity above the wall position $y = 0$. At each sampling time, we average $\eta(\partial v_x/\partial y)_{y=0}$ over all the fluid cells at the surface to obtain the fluid traction (shear stress) at the "resonator" surface. This leads to the impedance, as explained in the main text.

### Correspondence of units

To map the code units (c) with the International System of Units (SI) we start by selecting a reference length $\ell$. We have chosen $\ell = \delta/12$, which equals $\ell = 7.917$ nm for a penetration length of $\delta = 95$ nm, corresponding to 35 MHz. We note that the calculations presented in the main text were carried out with a grid size of $h = 0.5\ell$, corresponding to 24 fluid cells per $\delta$. The code units of mass $M$ and time $\tau$ match the density and kinematic viscosity of water at $T = 25^o$ C. In particular $M = \rho_c\ell^3$ follows from $\rho_c M/\ell^3 = \rho_{SI}$ kg/m$^3$ with $\rho_{SI} \approx 10^3$ (water) and we take $\rho_c = 1$. Choosing a value for the code's kinematic viscosity $\nu_c$ and matching the water kinematic viscosity $\nu_c\ell^2/\tau = \nu_{SI}$m$^2$/s yields the time scale $\tau$. From these fundamental units (mass, length and time), the code values for the QCM frequency $f_c$ and thermal energy $(k_BT)_c$ can be easily obtained. Table I shows these magnitudes and the units mapping used.

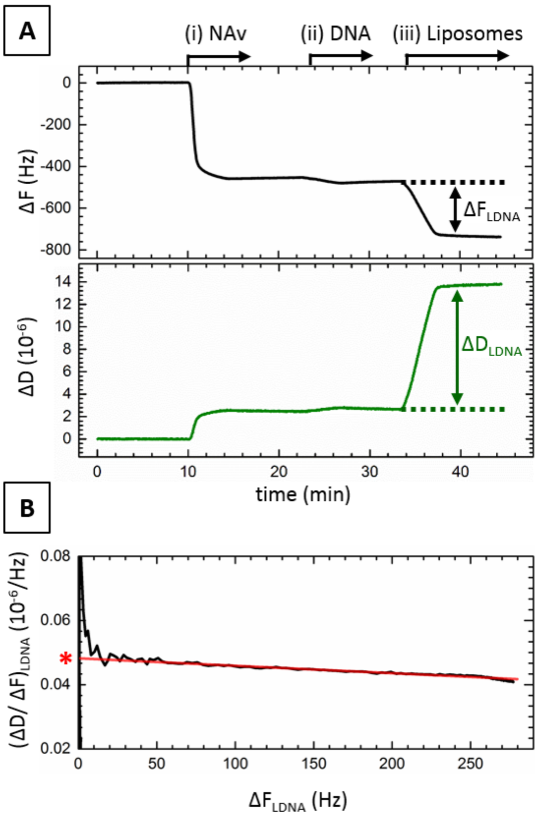


FIG. 1: Panel (A) shows a representative sensogram depicting binding events as recorded at 35 MHz (i.e., 7th harmonic) in real time: (i) neutravidin (0.2mg/mL) is adsorbed on the gold surface until saturation followed by (ii) the binding of biotinylated double stranded (ds) DNA (here 50 nM of 50 bp, i.e. 17 nm long) bearing a cholesterol at the opposite end; the latter can subsequently bind (iii) POPC liposomes (here 0.1 mg/mL of 25 nm radius). Frequency and dissipation changes registered upon addition of liposomes were used to calculate the acoustic ratio of the liposome-DNA (LDNA) complex as $\Delta D_{\rm LDNA}/\Delta f_{\rm LDNA}$. Panel (B) depicts a plot of this ratio $(\Delta D/\Delta f)_{\rm LDNA}$ against the corresponding frequency shift (proportional to the liposome surface coverage) during the formation of the LDNA complex, between minute 32 to minute 38 in panel (A). The dissipation capacity DC of the LDNA complex, defined as $\lim(\Delta D/\Delta f)_{\rm LDNA}$ when $\Delta f_{\rm LDNA} \to 0$, is marked with an asterisk.

### Molecular structures

*Liposomes*

Liposomes are modelled using the elastic network model (ENM). The membrane was created by beginning with a closed-packed arrangement of spheres connected to their nearest neighbours with harmonic springs. By changing the value of the spring constant, $k_L$, we could tune bending rigidity of the liposome membrane. In this work we consider $k_L = 100\,{\rm M}/\ell$, which corresponds to a quite rigid particle ($k_L\ell^2 > 10^5 k_BT$ for $T = 300$ K)). The size of the beads in the arrangement is fixed by the spatial resolution $h$ of the Eulerian fluid mesh. The calculations presented in the main text correspond to $h = 0.5\ell = 3.985$ nm. We used these connected spheres as building blocks for the membrane simply by selecting only the spheres contained between two concentric spheres with radii equal to the inner and outer radii of the liposome membrane. The number of beads required to build a liposome increases as $(R/h)^2$ being about 6000 beads for a liposome of radius $R = 50\,$nm.

TABLE I: Relation between code units and International System of units (SI), code and SI values of the parameters in simulation and equivalences between real and imaginary impedance $Z$ (code units) and frequency shifts $\Delta f$ (Hz) and dissipation factor $\Delta D$ for the $7^{th}$ harmonic of a quartz crystal with fundamental frequency $f_0 = 5$ MHz.

| **Magnitude** | **Code Units** | **SI units** |
|---|---|---|
| length | 1 | 7.917 nm |
| Mass | 1 | $4.96 \times 10^{-22}$ kg |
| Time | 1 | $1.416 \times 10^{-11}$ s |
| Kin. viscosity | 0.226 | $10^{-6}$ m$^2$/s |
| fluid density | 1 | $10^3$ kg/m$^3$ |
| sound velocity | 2.68 | $1.5 \times 10^3$ m/s |
| QCM frequency | 0.0005 | 35 MHz |
| $k_BT$ | $6.6 \times 10^{-5}$ | $4 \times 10^{-21}$ J |
| $Z_Q$ | 7.925 | $8.8 \times 10^6\,$kg/(m$^2$s) |
| Im[$Z$] | $10^{-3}$ | $\Delta f = 200.8\,$Hz |
| Re[$Z$] | $10^{-3}$ | $\Delta D = 1.826 \times 10^{-6}$ |

*DNA strand*

The DNA was modelled using the same type of beads as the liposome. The model reproduces a semiflexible polymer with bending rigidity

$$k_{bend} = k_BT(\ell_P/\sigma)$$

and persistence length $\ell_P = 50\,$nm evaluated at $k_BT = 4 \times 10^{-21}$ J (thermal energy at room temperature). It consists of a series of harmonic springs between consecutive beads (at distance $r = |\mathbf{R}_{i+1} - \mathbf{R}_i|$) with equilibrium distance $r_0 = \sigma$,

$$U_{sp}(r) = \frac{k_1}{2}(r - r_0)^2 \tag{1}$$

and a three body potential based on the angle $\theta$ between two consecutive bonds,

$$U_{angle}(r) = -\frac{k_{bend}}{2}\theta^2, \quad (2)$$

where we used $k_1 = 100$ to represent a almost unstreachable chain. We imposed an excluded volume interaction between DNA and liposome beads via the Weeks-Chandler-Anderson (WCA) potential (with excluded diameter $\sigma = 2h$). The DNA chain is connected to the liposome via an harmonic spring, so it is free to rotate. In practice, the range of angles formed between the DNA and the liposome tangent plane is slightly reduced due to the steric repulsion between beads (to about $[-70^o, 70^o]$). The other end of the DNA chain is linked to the QCM surface via a harmonic potential so that the chain is free to rotate at the linker point (corresponding to zero tilt energy). We checked that the tilt energy [7] at the linker-DNA connection slightly alters the liposome height distribution $P(y)$, but does not signficantly affect the acoustic ratio.

### Monte Carlo sampling of initial configurations and height probability density $P(y)$.

A pool of equilibrated initial configurations of individual liposome-DNA complexes was extracted from Monte Carlo (MC) sampling at $T = 300$ K. In these MC simulations, the liposome model was simplified to a single bead with radius $R$. The excluded volume interaction between the DNA beads and the single-bead liposome were modelled using a WCA potential (i.e. purely repulsive truncated Lennard-Jones potential) modified to be a function of the distance between the DNA bead and the liposome-surface, $r - \sigma_{eff}$ with $\sigma_{eff} = \sigma/2 + R$, where $r$ is the center-to-center distance, i.e.,

$$U_{EV}(r) = 4\epsilon\left[\left(\frac{r}{r_{i0} - \sigma_{eff}}\right)^{12} - \left(\frac{r}{r_{i0} - \sigma_{eff}}\right)^{6}\right]$$

with $\epsilon = 1$.

To accelerate the MC sampling we proceed as follows. i) The DNA bead-model is first generated by consecutively placing beads of radius $h$ at similar relative distances along a random walk with persistence 50 nm. The beads are placed such that their separation is given by the equilibrium distance ($r_0$) of the model (see Eq. 1). Details of this procedure are explained in Ref. [8]. This step is rejected if some bead crosses the wall (if $y_i < 0$) or if different beads in the chain overlap. ii) The liposome, constructed with a single bead of radius $R$, is then placed at a distance $R + h$ from the last DNA bead. The step is rejected if the liposome crosses the wall ($y < R$) or if some DNA bead crosses the outer liposome boundary (the distance between any DNA-bead and liposome center should be larger than $R + h$). The liposome-wall interaction was modelled as purely steric repulsion ($P(y) = 0$ for $y < R$). This choice is motivated by several observations: First electrostatic interactions with the wall are expected to be small because of the small charge of the neutravidin layer and the zero charge of POPC lipids (their zwiterionic head group is moreover strongly screened by the PBS saline buffer). Dispersion forces leading to physisorbtion were ruled out, upon comparision with experiments done with non-tethered liposomes. Simulations also confirmed that the acoustic response of adsorbed particles presents radically different trends when compared to suspended particles.

Longer MC runs were used to obtain the distribution of liposome distances $y$ above the resonator, $P(y)$, for various radii $R$ and DNA strands of contour length $L_{DNA}$. Results are plotted in Fig. 2 against the scaled distance $(y - R)/L_{DNA}$, which leads to a master curve.

## CONVERGENCE

*Stokes flow.* The base fluid impedance is needed to extract the analyte impedance ($\mathcal{Z}^{(\mathrm{LDNA})} = \mathcal{Z} - \mathcal{Z}^{(0)} - \mathcal{Z}^{(\mathrm{DNA})}$). A first check of the accuracy of the code is to compare the numerical and analytical values of the impedance of a Newtonian fluid, the latter given by the Gordon-Kanazawa result $\mathcal{Z}^{(0)} = \alpha\eta$ with $\alpha = (\mathrm{i} - 1)/\delta$. We used tall boxes (vertical direction $L_y \approx 5.3\delta$) for which the finite size correction to the fluid impedance is very small. As shown in Fig. 3, the relative deviation $(\mathcal{Z}_f^{(num)} - \mathcal{Z}^{(0)})/\mathcal{Z}^{(0)}$ between analytic and numerical fluid impedances is less or about $10^{-3}$ for $h = 0.5\,\ell$ (corresponding to $h/\delta = 1/24$ in the figure).

*Liposomes impedances.* Concerning the convergence of the liposome impedance, Fig. 3 (bottom panel), illustrates a study against the liposome-wall distance $y - R$ which compares results for $h = 7.917$ nm and $h = 3.985$ nm. The greater precision $h = 0.5\ell$ increases the resolution of the flow close to the wall, up to about distances of 4 nm.

## RESULTS FOR DNA

### Unloaded DNA tethers

To follow the experimental procedure, we extracted the contribution of the unloaded DNA strand $\mathcal{Z}^{(\mathrm{DNA})}$ from the total impedance, to obtain the pursued liposome-DNA impedance, i.e. $\mathcal{Z}^{(\mathrm{LDNA})} = \mathcal{Z} - \mathcal{Z}^{(0)} - \mathcal{Z}^{(\mathrm{DNA})}$. As in experiments, the impedance of dsDNA strands is much smaller than the liposome considered and single (unloaded) DNA strands (at the same coverage than as liposomes) will not be detected by the code resolution.

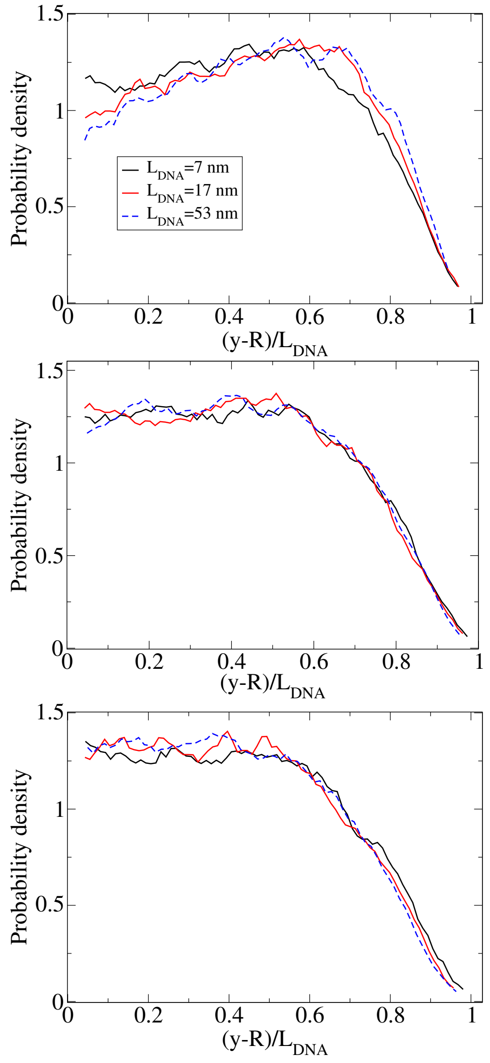


FIG. 2: Probability density for finding the liposome at height $y$ obtained from numerical calculations. From top to bottom, the liposome radius is $R = 15$, 50 and 100 nm. The liposomes are anchored to DNA chains of size $L_{DNA}$ and the interaction with the wall is purely due to steric repulsion.

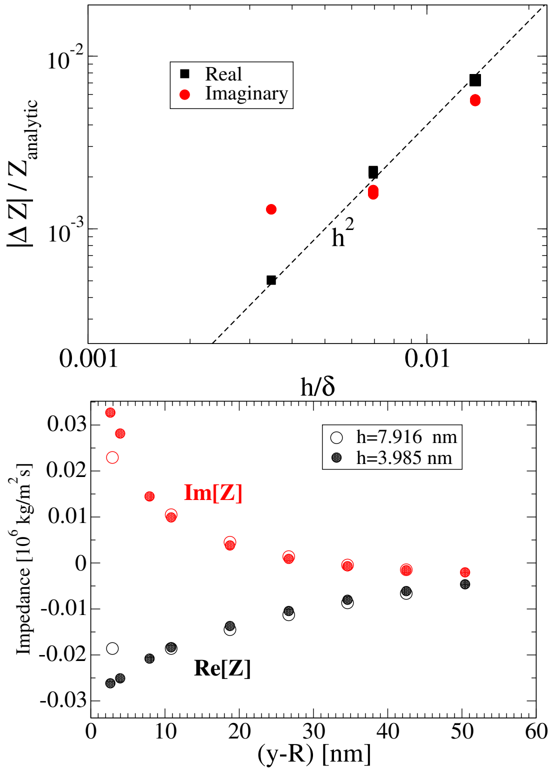


FIG. 3: (*Top*) Relative difference between the analytical $Z_{fluid} = (\mathrm{i} - 1)\eta/\delta$ and numerical value of the impedance of a Newtonian fluid versus the scaled mesh size $h/\delta$. (*Bottom*) The impedance of a freely suspended liposome of $R = 50$ nm obtained for two mesh resolutions $h$ as a function of the lipsome-wall (surface-to-surface) distance $y - R$.

Therefore we set a number $N_{DNA}$ of DNA strands, equilibrated according to the procedure in Sec.  on a smaller surface area $L^2$ (keeping $L_y = 5.3\delta$). In agreement with experiments [9] the scaled impedance $\mathcal{Z}^{(\mathrm{DNA})}/\phi$ is observed to be independent of the surface coverage, as shown in Fig. 4. Also in agreement with experiments, the DNA acoustic ratio was observed to increase with the DNA length as $\mathcal{A}^{(DNA)} \sim L_{DNA}^{\alpha}$, which is expected for short chains [9]. However, simulation values of $\mathcal{A}^{(DNA)}$ are about half the experimental ones. Quite probably, such differences arise from the limited spatial resolution we used here to model the DNA (with a bead diameter of about $h \approx 4$ nm). Note that in doing this DNA analysis, we need to use the same model as in the L-DNA simulations, so as to extract the DNA impedance from the the liposome-DNA impedance. A numerical study focusing on the QCM response of the DNA alone would certainly require smaller values of $h$ (finer resolution) and it is left for future effort.

**Impedances of anchored and free liposomes**

Figure 5 presents the results for the impedance of free liposomes at height $y$ $\mathcal{Z}^{(\mathrm{L})}(y)$ and liposomes cleaved to a DNA strand $\mathcal{Z}^{(\mathrm{LDNA})}$ at a similar distance from wall. Lines correspond to the ansatz in Eq. 1 of main text, which we also write here,

$$\mathcal{Z}^{(\mathrm{L})}(y) = Z_S\left[(A + \mathrm{i}B)\exp[-2\alpha y] + \frac{2\mathrm{i}C}{\alpha(y-R)}\right]. \quad (3)$$

with the stresslet impedance $Z_S = (20\pi/3)R^3\eta/(\delta^2 L^2)$ and $A \approx 1.40(R/\delta)^2$, $B \approx 1.5 - 0.03\exp(2.5\,R/\delta)$. The value of the constant $C$ obtained from the best fit to

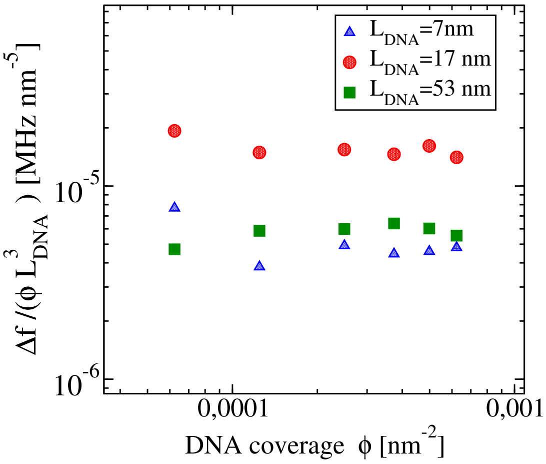


FIG. 4: Frequency shift created by DNA tethers divided by the DNA coverage $\phi = N_{DNA}/L^2$ for and scaled with $L^3_{DNA}$, against the coverage $\phi$. The dissipation is also almost independent of the coverage. The values of the acoustic ratio $-\Delta D/\Delta f$ (in MHz$^{-1}$ units) are $0.0185 \pm 0.005$ and $0.009 \pm 0.001$ respectively for $L_{DNA} = 53$ and 17 nm, which are about half the experimental values (0.03 and 0.018).

simulation values was found to depend slightly on $R$ (in particular, $C = 0.01$ for $R = 100$ nm, $C = 0.015$ for $R = 50$ nm and $C = 0.02$ for $R = 25$ nm). This fact is due to a resolution effect: we used a fixed value of $h$ so that the number of beads (of size $h$) used to resolve the liposome surface increases as $R^2$. In this sense, $R = 100$ nm corresponds to the best liposome resolution. The prediction of Eq. 2 of the main text (see Fig. 2 of main text), corresponds to $C = 0.01$ in Eq. 3 and it yields values of DC with are slightly closer to the experiments for $R < 100$ nm, compared with the numerical results obtained for fixed $h$

**Contribution of the DNA to the liposome-DNA impedance**

The contribution of the DNA to the liposome-DNA impedance was estimated as $\mathcal{Z}^{(\mathrm{LDNA})}_{DNA} = \mathcal{Z}^{(\mathrm{LDNA})} - \mathcal{Z}^{(\mathrm{L})}$ were $\mathcal{Z}^{(\mathrm{L})}$ is the impedance of a free liposome (without anchor). The average of $\mathcal{Z}^{(\mathrm{LDNA})}_{DNA}$ for different values of $y$ (liposome height) is plotted in Fig. 6 (error bars correspond to 1/3 of the standard deviation for 20 configurations). Results roughly scale as $\mathcal{Z}^{(\mathrm{LDNA})}_{DNA} \approx \left(-7.2\, R^{-2} + \mathrm{i}\, 83\, R^{-2.5}\right) L^{-0.5}_{DNA}\, Z_S$ (with $R$ and $L_{DNA}$ in nm).

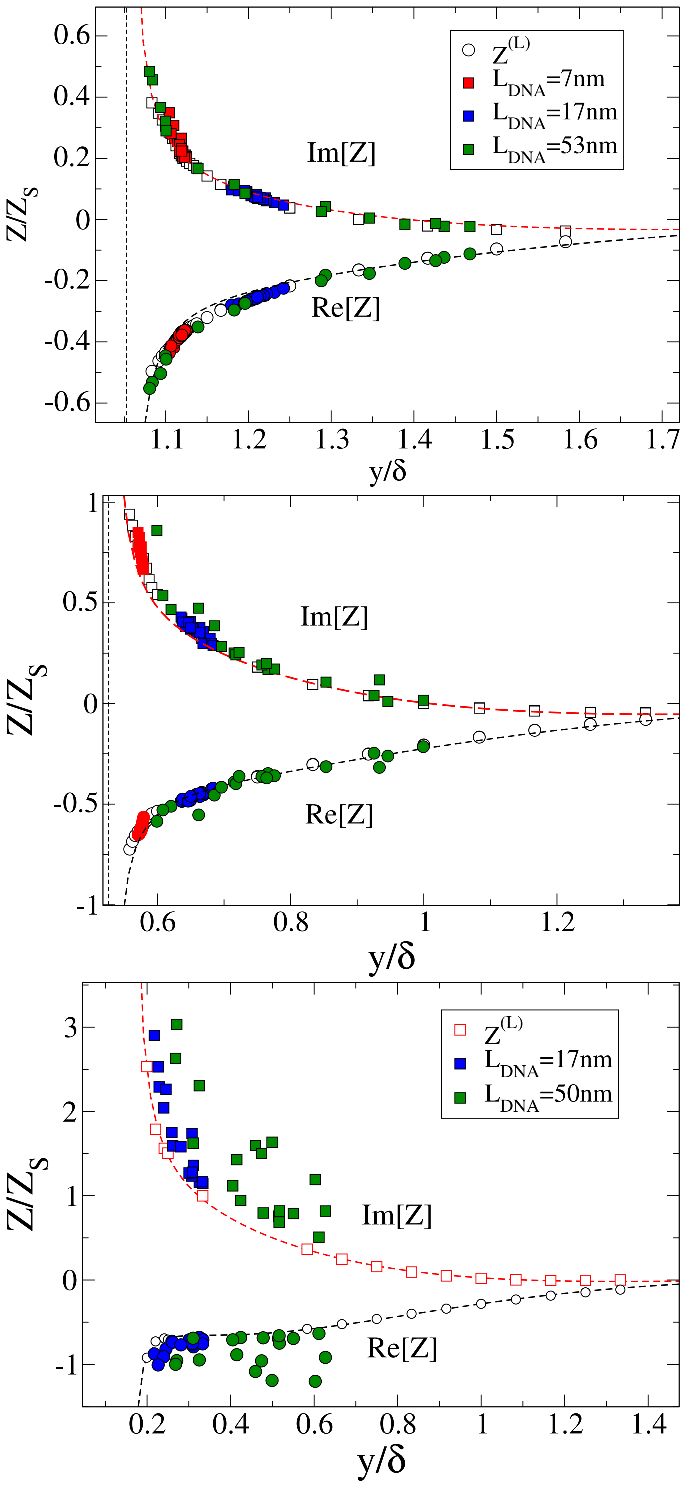


FIG. 5: The acoustic impedance of the liposome-DNA assembly $\mathcal{Z}^{(\mathrm{LDNA})}$ scaled with the stresslet impedance $Z_S = (20\pi/3) R^3 \eta/(\delta^2 L^2)$ for (top) $R = 100$ nm, $R = 50$ nm (middle) and 15 nm (bottom panel). Lines and open circles respectively correspond to numerical results and theoretical trend for a freely suspended liposome $\mathcal{Z}^{(\mathrm{L})}$ and filled symbols correspond to $\mathcal{Z}^{(\mathrm{LDNA})}$ for several lengths of the DNA strand. Results for $f_7 = 35$ MHz (for which $\delta = 95$ nm) in square boxes of side 506.67nm (in the $R = 15$ nm case, $L_x = L_z = 203.33$ nm). The spatial resolution is $h = \ell/2$ (with $\ell = 95/12$ nm).

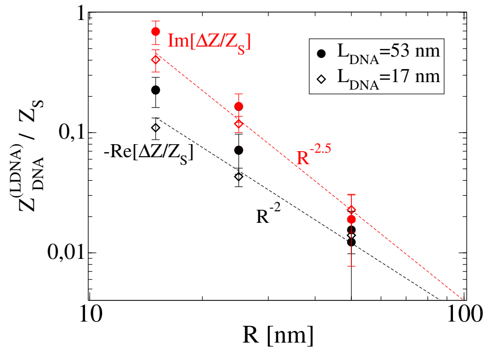


FIG. 6: Difference between the liposome-DNA complex impedance and that of a free liposome $\mathcal{Z}^{(\mathrm{LDNA})}_{DNA} \equiv (\mathcal{Z}^{(\mathrm{LDNA})} - \mathcal{Z}^{(\mathrm{L})})$, scaled with $Z_S = (20\pi/3)\eta R^3/(L^2\delta^2)$ (see main text). The error bars indicate *one third* of the standard deviation of $\mathcal{Z}^{(\mathrm{LDNA})}_{DNA}$ for 20 configurations.

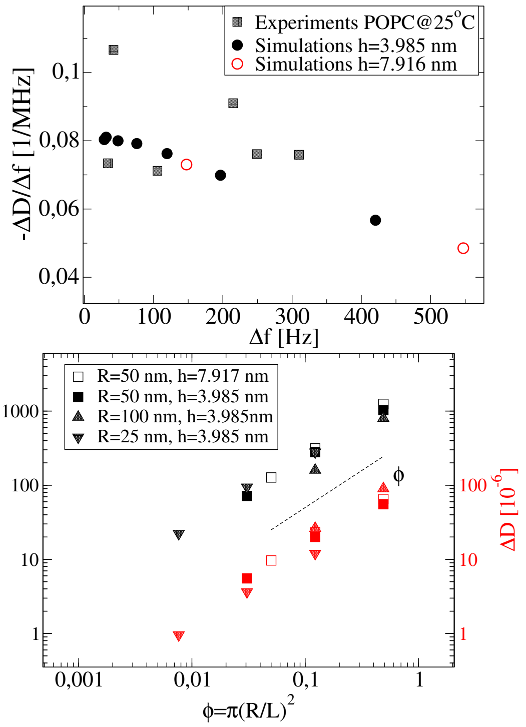


FIG. 7: (top panel) Acoustic ratio $-\Delta D/\Delta f$ (in $\mathrm{MHz}^{-1}$) versus frequency shift $\Delta f$ in Hz, for $L_{DNA} = 53$ nm (157 base pairs) and $R = 50$ nm comparing simulation results and experiments ($f_7 = 35$ MHz). Results obtained for a different spatial resolution $h$ are also shown. (bottom panel) $\Delta f$ and $\Delta D$ (dissipation factor) against the surface coverage, $\phi = \pi(R/L)^2$ corresponding to simulations for $L_{DNA} = 17$nm and different liposome radius and spatial resolution $h$.

**Effect of the liposome coverage (lateral box side).**

Figure 7 (top) compares simulation and experimental values of the ratio $-\Delta D/\Delta f$ with the frequency shift $\Delta f$. Both trends decay in a consistent fashion, despite the larger dispersion of experimental values for small coverage (small $\Delta f$). It is noted that modification in the spatial resolution $h$ leads to slight differences in the simulation values, which are however consistent with the overall trend. Figure 7 (bottom panel) shows $\Delta f$ and the dissipation factor $\Delta D$ against the liposome surface coverage $\phi = \pi(R/L)^2$. Results for two spatial resolutions $h$ have been included for liposomes of $R = 50$ nm radius, to illustrate the numerical convergence. Interestingly, $\Delta f$ and $\Delta D$ increases roughly linearly with $\phi$. Small deviations from linearity are found in the dissipation factor $\Delta D$, leading to the typical decrease of $-\Delta D/\Delta f$ against $\phi$ observed in experiments [10] when the same data is plotted against $\Delta f$. These subtle effects of coverage (non-linearity with $\phi$) are due to hydrodynamic interactions between large particles (liposomes, viruses) and it is not observed in unloaded DNA strands [9], nor in DNA-proteins assemblies [11]. However, a clear explanation of this effect is still lacking. We also expect that the details of $-\Delta D/\Delta f$ against $\phi$ will vary when considering an ensemble of particles at random locations.

---

* rafael.delgado@uam.es

[1] D. Milioni, P. Mateos-Gil, G. Papadakis, A. Tsortos, O. Sarlidou, and E. Gizeli, submitted (2020).
[2] F. B. Usabiaga, R. Delgado-Buscalioni, B. E. Griffith, and A. Donev, Computer Methods in Applied Mechanics and Engineering **269**, 139 (2014).
[3] F. B. Usabiaga, I. Pagonabarraga, and R. Delgado-Buscalioni, Journal of Computational Physics **235**, 701 (2013).
[4] F. B. Usabiaga, Ph.D. thesis, Universidad Autonoma de Madrid (2014).
[5] F. Balboa-Usabiaga, *FLUAM* `https://github.com/fbusabiaga/fluam/`.
[6] F. Balboa, J. B. Bell, R. Delgado-Buscalioni, A. Donev, T. G. Fai, B. E. Griffith, and C. S. Peskin, Multiscale Modeling & Simulation **10**, 1369 (2012).
[7] K.-Y. Wong and M. P. B., Biopolymers **73**, 570 (2004).
[8] N. Alcázar-Cano and R. Delgado-Buscalioni, Soft matter **14**, 9937 (2018).
[9] A. Tsortos, G. Papadakis, K. Mitsakakis, K. A. Melzak, and E. Gizeli, Biophysical journal **94**, 2706 (2008).
[10] D. Johannsmann, *The Quartz Crystal Microbalance in Soft Matter Research, Fundamentals and modeling* (Springer, 2015).
[11] D. Milioni, A. Tsortos, M. Velez, and E. Gizeli, Analytical chemistry **89**, 4198 (2017).
